# Supplementary material for: Weber's law based perception and the stability of animal groups
Source: arXiv:1806.00716 source file (2019-04-18)
Supplement: Supplementary file 1 [file Perna_Roy_Soc_Interface_supplementary_material_revised.pdf]

Electronic supplementary material

# Weber's law based perception and the stability of animal groups

Andrea Perna[1,2], Giulio Facchini[1], Jean Louis Deneubourg[2]
[1] *Life Sciences Department, University of Roehampton, London, UK*
[2] *Unit of Social Ecology, Université Libre de Bruxelles, Bruxelles, Belgium*

## S1 Derivation of the continuous diffusion equation.

The continuous diffusion equation:

$$\frac{\partial C}{\partial t} = D' \frac{\partial^2 C}{\partial x^2} \tag{S1}$$

can be derived from the discrete equation

$$\begin{aligned} C(x, t + \Delta t) = \\ C(x,t) + D\left[-2C(x,t) + C(x+\Delta x, t) + C(x - \Delta x, t)\right] \end{aligned} \tag{S2}$$

by considering the Taylor series approximation of $C(x, t + \Delta t)$ around $C(x, t)$:
$C(x, t + \Delta t) = C(x, t) + \Delta t \frac{\partial C}{\partial t} + ...$
and the Taylor series approximation of $C(x + \Delta x, t)$ around $C(x, t)$:
$C(x + \Delta x, t) = C(x, t) + \Delta x \frac{\partial C}{\partial x} + \frac{(\Delta x)^2}{2} \frac{\partial^2 C}{\partial x^2} + ....$
When these are plugged into equation S2, the first spatial derivatives cancel each other out and the remaining equation is $\Delta t \frac{\partial C}{\partial t} = D(\Delta x)^2 \frac{\partial^2 C}{\partial x^2}$. We then collect the parameters $\Delta t$, $D$ and $(\Delta x)^2$ into a new constant $D'$.

## S2 A training problem: recovering Gaussian distributions.

Imagine to release a certain number of animals at a single location ($C(x, 0)$ is a delta function). Equation 3 of the main text tells us that, in the absence of *any* interactions, after some time $t$ the individuals will be distributed according to a Gaussian distribution $G$ centered around the release point and whose variance is proportional to $t$.

One first question that we can ask is, what kind of movement response would allow the group to temporarily contrast the spreading process and revert from the spatial distribution that was produced at time $t$ to the distribution that existed before, at time $t - \Delta t$ (fig. S1)

In this simple case comes to our help the fact that we just want to convert a Gaussian distribution (the distribution at time $t$; dotted distribution in figure S1) into another Gaussian distribution (that existed at some previous time $t - \Delta t$ (shaded distribution in figure S1). The simplest way in which this can be achieved is if each individual moves

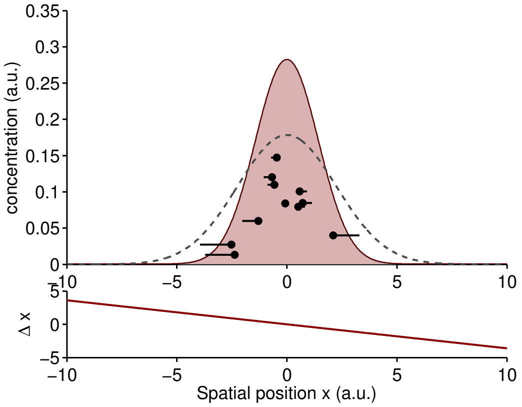


**Figure S1. Individual movements to contrast gaussian diffusion. (Top)** diffusion transforms a Gaussian distribution (continuous shaded curve) into a scaled version of the same distribution (dashed curve). In order to restore the original distribution, the particles that form the distribution (visually illustrated as black dots in the figure) must move towards the origin.**(Bottom)** The distribution resulting from the movement of particles remains Gaussian if the movement of particles towards the origin ($\Delta x$) is directly proportional to the distance from the origin ($x$) of the particles themselves.

towards the direction of higher local density by an amount $\Delta x$ proportional to its own current distance $x$ from the centre of the distribution.

In practice, however, we should assume that individuals do not have a global perception, that is, they do not know directly their own position relative to the centre of the distribution. They can, however, estimate the number of neighbours locally around their own position and its local variation in different directions. In the case of Gaussian distributions, it is easy to verify that there is one function of these local quantities that is proportional to the distance from the centre of the distribution: this is the gradient normalized over the local density $x = -\frac{\nabla G}{G}\sigma^2$, where $\nabla G = \frac{\partial G}{\partial x}$ indicates the gradient of the Gaussian distribution (because $\frac{\partial G}{\partial x} = -\frac{x}{\sigma^2}G$). Expressions of the form $\frac{\nabla f}{f}$ are well known in psychophysics and correspond to Weber's law.

## S3 Non-linear probability of response

Equation 5 in the main text describes the probability for an individual to move towards a higher concentration region as increasing linearly with the Weber's fraction $w$ of local concentrations:

$$p(x \to x + \Delta x) = \gamma w \tag{S3}$$

with

$$w = \frac{|C(x + \Delta x) - C(x)|}{C(x)} \tag{S4}$$

being the Weber's fraction and $\gamma$ a proportionality constant (Weber's coefficient).

This formulation is clearly a simplification as real probabilities need to deviate from linearity for large values of the Weber's fraction (they cannot become larger than one) and

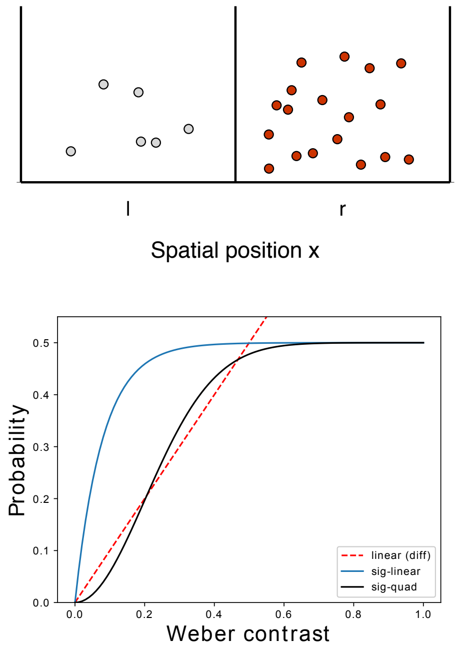


**Figure S2. Non-linear Weber's law response in a two-cells model.** (Top) Particles move between two cells. (Bottom) Each particle responds to the gradient of concentration with an increasing probability of moving towards the cell with higher concentration. This probability can increase linearly (red dashed line), or sigmoidally (continuous blue and black lines). Blue line: asymptotically linear equation S6; black line: asymptotically quadratic S7. All probabilities are scaled to a maximum of 0.5

real psychophysical responses typically have a logistic shape.

In this section we consider briefly the case of probabilities increasing as a non-linear function $F$ of Weber's fraction:

$$p(x \to x + \Delta x) = F(\gamma w) \tag{S5}$$

and we focus in particular on a sigmoid response function that is asymptotically linear

$$F(\gamma w) = 1 - \exp(-\gamma w) \tag{S6}$$

and an asymptotically quadratic sigmoid response function:

$$F(\gamma w) = 1 - \exp(-\gamma w^2) \tag{S7}$$

We consider the case scenario of particles moving between two cells. Each particle has a constant probability of moving to the adjacent cell by diffusion and also experiences a probability of moving towards the cell with higher concentration that depends on the Weber's fraction of the two concentrations (fig. S2).

When the argument of $F$ is small, the function in equation S6 is linear, but it progressively deviates from linearity when the argument becomes larger. This deviation from linearity has implications for the long-term evolution of the system resulting from the

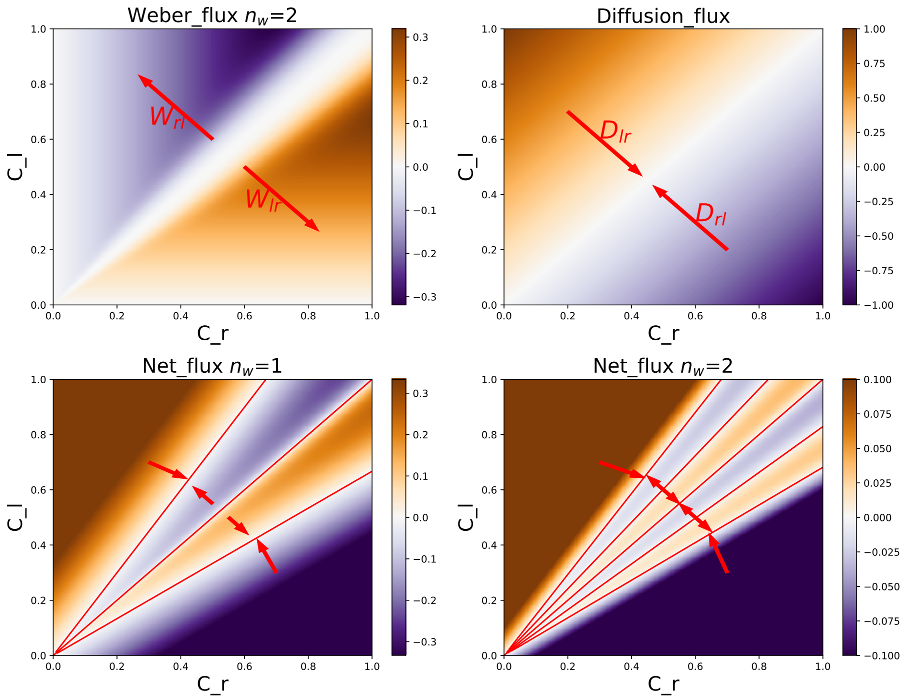


**Figure S3. Equilibrium points of non-linear Weber's law models with two cells.** (Top-left) Gradient response based on a non-linear Weber's law (as in eq. S7) produces a flux from the cell with lower concentration to the cell with higher concentration. (Top-right) Diffusion produces a flux from the cell with higher to the lower concentration. (Bottom-left) Gradient response based on asymptotically linear sigmoid response (eq. S6) and diffusion interact together to produce a stable equilibrium for a constant ratio of concentration. (Bottom-right) When the gradient response is an asymptotically quadratic sigmoid function, also the homogeneous state becomes stable. Cl: left cell; Cr: right cell; Wrl: Weber flux from right to left; Wlr: Weber flux from left to right; Dlr: diffusion flux from left to right; Drl: diffusion flux from right to left. In all these models the anti-diffusion coefficient $\gamma$ is intended to be larger than the diffusion coefficient $D$. For this particular figure $\gamma = 12.5D$.

contrasting effects of diffusion and gradient response (fig. S3). In fact, a purely linear Weber's law response, such as in equation S3, combines with diffusion to simply produce a slower diffusion (the concentrations in the two cells eventually level out) or an anti-diffusion (all particles eventually migrate to one single cell). Conversely, in the case of the sigmoidal Weber's law response of equation S6 (asymptotically linear sigmoid response), gradient response and diffusion can balance each other out to generate a non-homogeneous equilibrium which stabilises a constant concentration ratio (fig. S3). With the non-linear equation S7 (asymptotically quadratic sigmoid response) both a constant concentration ratio and the homogeneous state become stable equilibrium points.

These simple analyses indicate that while a sigmoid Weber's law response would be very similar to the linear model considered in the main text, the deviations from linearity could contribute to determine the profile of concentration emerging in a group when anti-diffusion forces are stronger than diffusion. Specifically, at the location of steep edges of concentration the anti-diffusion flux produced by Weber's law response is no longer

sufficient to contrast diffusion. While this difference only has a relatively small impact on small-scale diffusion and anti-diffusion phenomena such as those illustrated in figure 2 in the main text, it would have the potential to shape the long-term equilibrium of the system if Weber's law were the only 'social force' acting on the system.

## S4 Internal movements within a Gaussian probability landscape that remains stable over time.

Here we consider a Gaussian distribution stable over time, and we assume that individuals move freely within this distribution. The global distribution does not change, but there are internal movements inside this distribution.

Individual trajectories are generated as sequences of multivariate random normal numbers with covariance matrix

$$C = \lambda^2 \exp(-\frac{(i-j)^2}{\eta^2}) \tag{S8}$$

where $\lambda = 1$ determines the variance of the simulated distribution and $\eta = 10$ controls the correlation length, while $i$ and $j$ are the indices of matrix elements. Different values of these parameters do not affect the qualitative nature of this example. One such trajectory is illustrated in figure S4(a), and the probability density of all these trajectories converges to the distribution in figure S4(b).

When the movement of particles in these simulated trajectories is described in terms of the average change of position $\Delta x$ for a given starting position $x$ we observe a clear linear regression in which more peripheral particles on average tend to move towards the centre of the distribution. If this average movement is expressed not in terms of the absolute position of the particle, but in terms of the local distribution density and gradient we find the Weber's law type of response described in the previous sections of this document.

## S5 Movements within stable density landscapes: details of methods

In order to explore the interaction responses compatible with maintaining a stable density landscape we first created random density landscapes and then we simulated movements of particles over each landscape while imposing that the flows of particles in alternate directions over each edge is balanced for each time step.

The random density landscapes were obtained as low-pass filtered two-dimensional noise: we first created a 2D array of random values uniformly distributed within a given range and then we removed high spatial frequencies by convolving with a two-dimensional Gaussian distribution). We tested multiple landscapes with different values of average density, amplitude of modulation and spectral composition.

The probability for an individual particle to move from a cell $i$ to an adjacent cell $j$ was calculated as follows: first we calculated the flows of particles that would move from $i$ to $j$ through diffusion alone, $F_{ij}^{fwd} = DN_i$. Then we immediately compensated these flows by moving an identical number of particles in the opposite direction. These particles are selected randomly among those available in $j$ and could be the same that had just moved from $i$ to $j$ with probability $F_{ij}^{fwd}/(F_{ij}^{fwd} + N_j)$. As a result, the net flow of particles that moved from $i$ to $j$ because of diffusion and were not put back during the compensatory

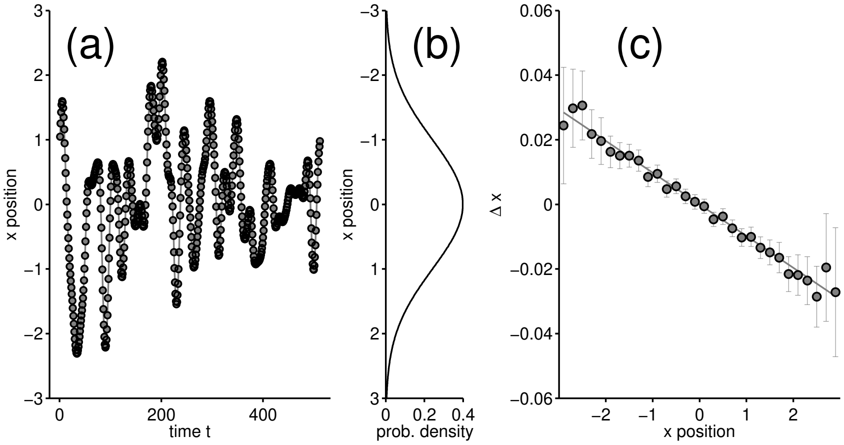


**Figure S4. Apparent Weber's law response of randomly moving particles in a Gaussian density distribution.** (a) Simulated x position of a particle that moves randomly across a Gaussian probability landscape. depicted in (b). (c) Average movement (± standard deviation) of a particle as a function of its current position. Individual particles are observed to move towards the centre of the distribution with a step length directly proportional to their current distance from the centre of the distribution.

step is $FD_{ij} = F_{ij}^{fwd} - (F_{ij}^{fwd})^2/(F_{ij}^{fwd} + N_j)$, and it is associated with a net compensatory flow from $j$ to $i$, $FC_{ji} = FD_{ij}$. By imagining that the same process also takes place in the opposite direction, with diffusion from $j$ to $i$, and a compensatory movement from $i$ to $j$, the total flow between $i$ and $j$ is $FD_{ij} + FCij$ .

## S6 Amplification and attenuation of different spatial harmonics around the homogeneous state

We consider the evolution of $C$ around an homogeneous steady state where a small perturbation $\delta$ is applied: $C(x,t) = C_s + \delta(x,t)$. We choose a form for $\delta = e^{\omega t} e^{ikx}$ which allows us monitoring the temporal and spatial evolution of the perturbation.

If diffusion and anti-diffusion act simultaneously, we have:

$$\frac{\partial C}{\partial t} = +D\frac{\partial^2 C}{\partial x^2} - \gamma\frac{\partial^2 C}{\partial x^2} \tag{S9}$$

The equation implies an immediate response of individuals to the diffusion event, so that in practice it is equivalent to a slower diffusion (if $D > \gamma$) or slow anti-diffusion (if $\gamma > D$).

The time derivative in equation S9 can be rewritten around the homogeneous state as $\frac{\partial C}{\partial t} = \left(\frac{\partial C_s}{\partial t} + \frac{\partial \delta(x,t)}{\partial t}\right)$, and similarly for the space derivative $\frac{\partial^2 C}{\partial x^2} = \left(\frac{\partial^2 C_s}{\partial x^2} + \frac{\partial^2 \delta(x,t)}{\partial x^2}\right)$. As the derivative of the constant parts are equal to zero, equation S9 around the homogeneous state becomes

$$\frac{\partial \delta}{\partial t} = (D-\gamma)\frac{\partial^2 \delta}{\partial x^2}$$

from which we have $\omega\delta = (D-\gamma) - k^2\delta$ which indicates that the speed $\omega$ at which harmonics of a given frequency $k$ are amplified or attenuated (depending on the sign of

$D - \gamma$) is proportional to the square of the frequency: high frequency harmonics are both amplified faster when anti-diffusion prevails and attenuated faster when diffusion prevails.
